# Supplementary material for: Concept Replacer: Replacing Sensitive Concepts in Diffusion Models via Precision Localization
Source: arXiv:2412.01244 source file (2024-12-03)
Supplement: Supplementary file 1 [file X_suppl.tex]

\clearpage
\maketitlesupplementary

\section{Ablation Study}
\label{sec:Ablation Study}

\section{Additinoal Results on Concept Location and Replacing}
\label{sec:Location}
